# Supplementary material for: Issues with Input-Space Representation in Nonlinear Data-Based Dissipativity Estimation
Source: arXiv:2411.13404 source file (2024-11-20)
Supplement: Supplementary file 1 [file AppendixB.tex]

Consider a Fourier basis, with $b,T<\infty$. That is, for all $u\in\mathcal{U}$, there exist constants $\alpha_i$ such that $u(t) = \sum_{i=1}^b \alpha_iv_i$, where $v_i = v'_i/\|v'_i\|$, and $v'_i = \cos(\frac{2\pi i}{T}t)$. This way, $v_i$ are orthonormal to each other. Also define $\omega_i = \frac{2\pi i}{T}$ (Note, I'm using $i$ as an index, not the imaginary; that will be $j=\sqrt{-1}$). Let $\widehat{(\cdot)}$ denote the Fourier transform. Then for a linear system, $G$,
\begin{align}
    2\pi\|Gu\| &= \|\hat{G}\hat{u}\| \\
    &= \|\hat{G}\int_{-\infty}^\infty u(t)e^{-j\omega t}dt\| \\
    &= \|\hat{G}\int_{-\infty}^\infty \sum_{i=1}^b\alpha_iv_i(t) e^{-j\omega t}dt\| \\
    &= \|\sum_{i=1}^b\alpha_i\hat{G}\int_{-\infty}^\infty \frac{v'_i(t)}{\|v_i\|} e^{-j\omega t}dt\| \\
     &= \|\sum_{i=1}^b\frac{\alpha_i}{\|v_i\|}\hat{G} \pi\left(\delta(\omega-\omega_i) + \delta(\omega+\omega_i)\right)\| \\
    &= \|\pi\sum_{i=1}^b\frac{\alpha_i}{\|v_i\|} \hat{G}\delta(\omega-\omega_i) + \pi\sum_{i=1}^b\frac{\alpha_i}{\|v_i\|} \hat{G}\delta(\omega+\omega_i)\| \\
     &\leq \pi\sum_{i=1}^b\|\frac{\alpha_i}{\|v_i\|} \hat{G}\delta(\omega-\omega_i)\| + \pi\sum_{i=1}^b\|\frac{\alpha_i}{\|v_i\|} \hat{G}\delta(\omega+\omega_i)\| \\
    &\leq 2\pi\sum_{i=1}^b\|\frac{\alpha_i}{\|v_i\|} \hat{G}\delta(\omega-\omega_i)\| \\
    &\leq 2\pi\sum_{i=1}^b|\frac{\alpha_i}{\|v_i\|}|\|\hat{G}\delta(\omega-\omega_i)\| \\
    &\leq 2\pi\sum_{i=1}^b|\frac{\alpha_i}{\|v_i\|}|\gamma_{\omega_i} 
    %\hat{y}(\hat{u}) &= \sum_{i=1}^b\alpha_i\hat{G}\hat{v}_i \\
    %\hat{y}(\hat{u})&= \sum_{i=1}^b\alpha_i\hat{y}(\hat{v}_i) \\
    %y(u) &= \sum_{i=1}^b\alpha_i y(v_i) \\
    %\|y(u)\| &= \norm{\sum_{i=1}^b\alpha_iy(v_i)} \\
     %\|y(u)\| &= \norm{\sum_{i=1}^b\alpha_iy\left(\frac{\cos(\omega_i t)}{\|\cos(\omega_i t)\|}\right)} \\
     %&\leq \sum_{i=1}^b\norm{\alpha_iy\left(\frac{\cos(\omega_i t)}{\|\cos(\omega_i t)\|}\right)}
\end{align}
Where (12) is from Parseval's theorem, (13) is from Fourier transform, (16) is from Fourier transform of cosine, (18) and (19) are from Triangle Inequality, (20) is from Cauchy-Schwartz, and $\gamma_{\omega_i}$ is the gain response of $G$ at $\omega_i$. Therefore, $\|Gu\|\leq \sum_{i=1}^b|\nicefrac{\alpha_i}{\|v_i\|}|\gamma_{\omega_i}$, which is the weighted average of the gain at each basis frequency. Therefore, the system can never have a gain outside of the maximum and minimum attained by the basis frequencies, no matter how many samples are taken.

Now consider any other orthogonal basis, $v'_i$. It can be represented by a Fourier series, $v'_i = \sum_{k=0}^\infty \beta_{i,k}\cos(\omega_k t)$. Picking up from (15), 
\begin{align}
    2\pi\|Gu\| &= \|\sum_{i=1}^b\alpha_i\hat{G}\int_{-\infty}^\infty \frac{v'_i(t)}{\|v_i\|} e^{-j\omega t}dt\| \\
     &= \|\sum_{i=1}^b\alpha_i\hat{G}\int_{-\infty}^\infty \frac{\sum_{k=0}^\infty \beta_{i,k}\cos(\omega_k t)}{\|v_i\|} e^{-j\omega t}dt\| \\
     &= \|\sum_{k=0}^\infty\left(\sum_{i=1}^b\frac{\alpha_i}{\|v_i\|} \beta_{i,k}\right)\hat{G}\int_{-\infty}^\infty \cos(\omega_k t) e^{-j\omega t}dt\| 
\end{align}
skipping ahead,
\begin{align}
    \|Gu\| &\leq  \sum_{k=0}^\infty\left(\sum_{i=1}^b|\frac{\alpha_i}{\|v_i\|} \beta_{i,k}|\right)\gamma_{\omega_k}
\end{align}
or
\begin{align}
    \|Gu\| &\leq  \sum_{i=1}^b|\frac{\alpha_i}{\|v_i\|}|\left(\sum_{k=0}^\infty |\beta_{i,k}|\gamma_{\omega_k}\right)
\end{align}
I neglected the potential phase shift, but I believe it doesn't matter. Now we have the weighted average over each basis function, and the weighted average over the relative frequency contribution of each basis function. Even though potentially infinite frequencies are represented by a basis function, we only see the response to the weighted average of those frequencies in the output. (Better explanation below).

\textbf{Tighter statement to put in the paper}

Consider an LTI system, $G:\mathcal{U}_{A234}\rightarrow \mathcal{Y}$, and an orthonormal Fourier basis for $\mathcal{U}_{A1234}$ with $b,T<\infty$. For all $u\in\mathcal{U}$, there exists $\alpha_i$ such that $u(t)=\sum_{i=1}^b \alpha_iv_i$, where $v_i = v_i'/\|v_i'\|$, $v_i' = \cos(\omega_it)$, and $\omega_i = \frac{2\pi i}{T}$. Let the gain response of $G$ to a sinusoid of frequency $\omega_i$ be denoted $\gamma_{\omega_i}$. Let $\gamma_{max} \defeq \max_i \gamma_{\omega_i}$, $\omega_{max} \degeq \arg\min \gamma_{\omega_i}$ and likewise for $\gamma_{min}$ and $\omega_{min}$. Let the Fourier transform be denoted $\hat{(\cdot)}$. By applying the Fourier transform and using linearity of the operator, it may be shown that $\|Gu\| = \frac{1}{2\pi}\|\hat{G}\hat{u}\| \leq \sum_{i=1}^b|\nicefrac{\alpha_i}{\|v_i\|}|\gamma_{\omega_i}$, which is a weighted average of the gain responses at each basis frequency. Therefore, the extremum gain responses are achieved by sampling each basis independently, and every additional sample is redundant. Further, if $\omega_{max}$ and $\omega_{min}$ are not sampled frequencies, then $\gamma_{max}$ and $\gamma_{min}$ will never be realized in the data. 

Any other orthonormal basis can be represented as a Fourier series, as in $v_i' = \sum_{k=0}^\infty \beta_{i,k}\cos(\omega_k t + \theta_k)$. It can then be shown that $\|Gu\| \leq  \sum_{i=1}^b|\frac{\alpha_i}{\|v_i\|}|\left(\sum_{k=0}^\infty |\beta_{i,k}|\gamma_{\omega_k}\right)$. Now, the weighted average is taken over the frequency components of the basis functions' Fourier series. Again, the extremum values in the data are obtained by sampling each basis independently, and additional samples merely interpolate. Even if a basis contains a nonzero component of $\omega_{max}$ or $\omega_{min}$, it will be averaged with non-extremum values, so $\gamma_{max}$ and $\gamma_{min}$ will not be attained.
